# Supplementary material for: Efficient sampling of spreading processes on complex networks using a composition and rejection algorithm
Source: arXiv:1808.05859 source file (2019-02-11)
Supplement: Supplementary file 1 [file sm.pdf]

# Efficient sampling of spreading processes on complex networks using a composition and rejection algorithm : supplementary material

Guillaume St-Onge,[1,2,*] Jean-Gabriel Young,[1,2] Laurent Hébert-Dufresne,[1,3] and Louis J. Dubé[1,2]

[1] *Département de Physique, de Génie Physique, et d'Optique, Université Laval, Québec (Québec), Canada, G1V 0A6*

[2] *Centre interdisciplinaire de modélisation mathématique de l'Université Laval, Québec (Québec), Canada, G1V 0A6*

[3] *Department of Computer Science and Vermont Complex Systems Center, University of Vermont, Burlington, VT 05401, USA*

(Dated: January 30, 2019)

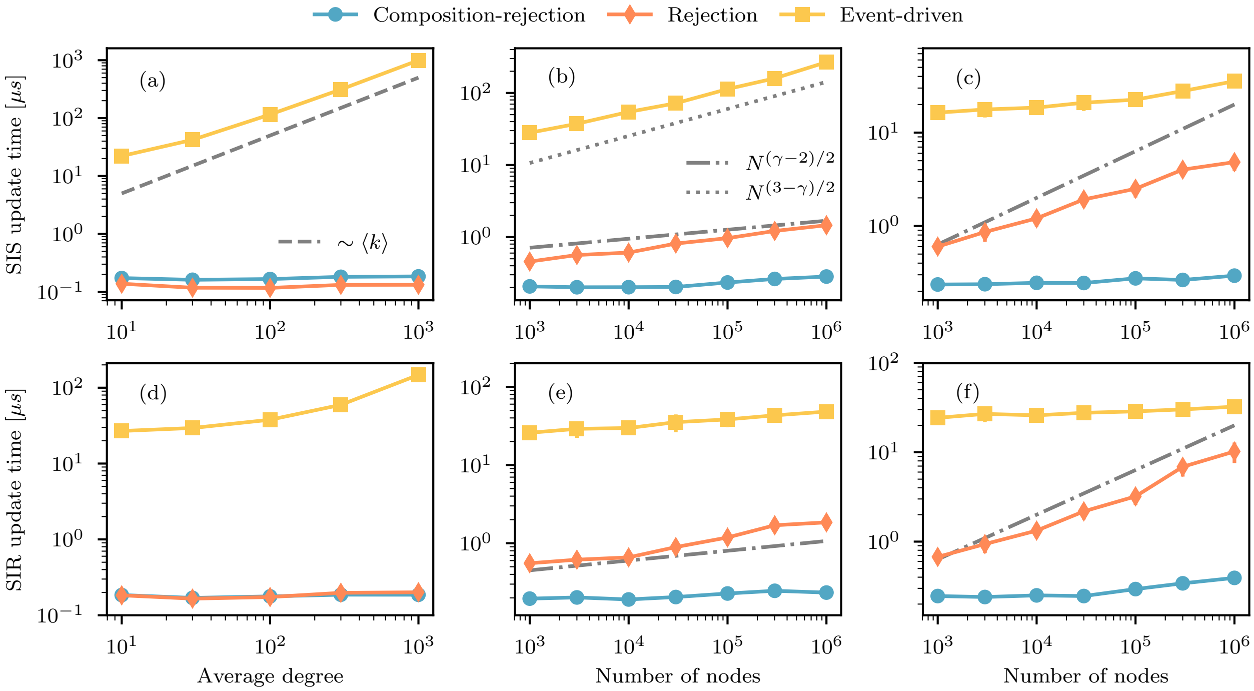


FIG. S1. Absolute average computation time for a single update of the state for spreading processes using different algorithms. Each marker is averaged over 10 simulations on 10 realizations of a random graph ensemble. The rejection and composition and rejection methods are implemented in C++, while the event-driven method is implemented in Python. **(Upper row)** Average over sequences of $10^6$ state transitions for the SIS model in the stationary state. The systems have been thermalized using $10^6$ transitions beforehand. **(Lower row)** Average over $10^6/N$ complete sequences of the SIR model, starting with an initial infected node density of $10^{-2}$. **(a)** and **(d)** $G(N, M)$ random graphs with fixed number of nodes $N = 10^4$ and different average degree $\langle k \rangle$. The recovery and transmission rates used are $\mu = 1$ and $\lambda = 1.05\lambda_c$ . **(b)** and **(e)** Random graphs with an expected degree sequence [1, 2]. We used a power law expected degree distribution $P(\kappa) \sim \kappa^{-\gamma}$ with $\gamma = 2.25$, $\kappa_{\min} = 3$ and $\kappa_{\max} < \langle k \rangle N^{1/2}$. The recovery and transmission rates used are $\mu = 1$ and $\lambda = 3\lambda_c$. **(c)** and **(f)** Same as (b) and (e), but with $\gamma = 3$.

* guillaume.st-onge.4@ulaval.ca

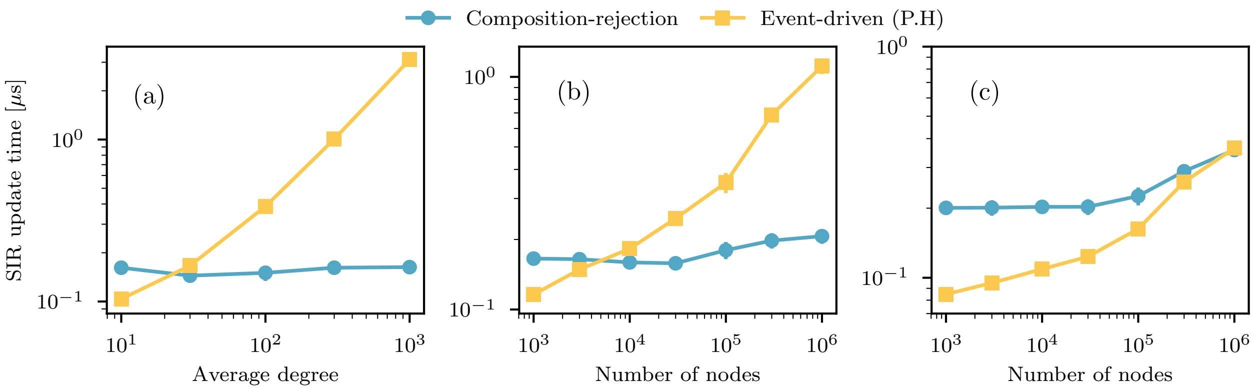


FIG. S2. Average computation time for a single update of the state for the SIR model using different algorithms. Each marker is averaged over 10 simulations on 10 realizations of a random graph ensemble. The composition and rejection method is implemented in C++ and the event-driven method of Ref. [4] is implemented in C. Averages are performed over $10^6/N$ complete sequences of the SIR model, starting with an initial infected node density of $10^{-2}$. **(a)** $G(N, M)$ random graphs with fixed number of nodes $N = 10^4$ and different average degree $\langle k \rangle$. The recovery and transmission rates used are $\mu = 1$ and $\lambda = 1.05\lambda_c$ . **(b)** Random graphs with an expected degree sequence [1, 2]. We used a power law expected degree distribution $P(\kappa) \sim \kappa^{-\gamma}$ with $\gamma = 2.25$, $\kappa_{\min} = 3$ and $\kappa_{\max} < \langle k \rangle N^{1/2}$. The recovery and transmission rates used are $\mu = 1$ and $\lambda = 3\lambda_c$. **(c)** Same as (b), but with $\gamma = 3$.

## I. COMPUTATION TIME COMPARISON WITHOUT RESCALING

To facilitate the comparison of various methods across different programming languages, we have rescaled by a constant factor the computation time of the event-driven method (Fig. 4 in the main text). Supplementary Fig. S1 shows a comparison of the methods without rescaling.

## II. ADDITIONAL COMPUTATION TIME COMPARISON FOR THE SIR MODEL

The decision to compare our method with the package of Ref. [3] is mainly due to the fact that it provides a user-friendly interface, both for the SIS and the SIR. However, the difference in programming language obfuscates the comparison of the absolute computation time, as it mostly reveals the difference in efficiency of the compiled code. Supplementary Fig. S2 provides a comparison of the computation time between our method and that of Petter Holme [4], an event-driven algorithm for the SIR model. We can see that both methods are competitive, ours being preferable for dense or large and heterogeneous networks.

---


[1] F. Chung and L. Lu, Annals of Combinatorics **6**, 125 (2002).

[2] J. C. Miller and A. Hagberg, in *Algorithms and Models for the Web Graph*, edited by A. Frieze, P. Horn, and P. Prałat (Springer Berlin Heidelberg, Berlin, Heidelberg, 2011) pp. 115–126.

[3] I. Z. Kiss, J. C. Miller, and P. L. Simon, *Mathematics of Epidemics on Networks: From Exact to Approximate Models*, Vol. 46 (Springer, 2017).

[4] P. Holme, "sir," `https://github.com/pholme/sir` (2018).
